# Supplementary material for: SimPLR: A Simple and Plain Transformer for Efficient Object Detection and Segmentation
Source: arXiv:2310.05920 source file (2025-03-13)
Supplement: Supplementary file 1 [file additional.tex]

\section{Additional Results}

\begin{table}[h]
    \centering
    \footnotesize
    % \floatbox[{\capbeside\thisfloatsetup{capbesideposition={top,right}}}]{table}[\FBwidth]
    {
    \tablestyle{4.5pt}{1.2}
    \begin{tabular}{lcccccc}
    \multicolumn{1}{l|}{method} & backbone & \multicolumn{1}{c|}{pre-train} & PQ & PQ$^\text{th}$ & \multicolumn{1}{c|}{PQ$^\text{st}$} & FPS \\
    \shline
    \rowcolor{orange!50} \textbf{Feature pyramids} &  &  &  &  &  &  \\
    \multicolumn{1}{l|}{MaskFormer~\citep{cheng2021maskformer}} & Swin-B & \multicolumn{1}{c|}{sup-1K} & 51.1 & 56.3 & \multicolumn{1}{c|}{43.2} & - \\
    \multicolumn{1}{l|}{Mask2Former~\citep{cheng2022mask2former}} & Swin-B & \multicolumn{1}{c|}{sup-1K} & 55.1 & 61.0 & \multicolumn{1}{c|}{46.1} & 7 \\
    \hline
    \rowcolor{orange!50} \textbf{Plain detector} &  &  &  &  &  &  \\
    \multicolumn{1}{l|}{\ours} & ViT-B & \multicolumn{1}{c|}{sup-1K} & \textbf{55.5} & \textbf{61.4} & \multicolumn{1}{c|}{\textbf{46.2}} & \textbf{13} \\
    \end{tabular}
    }
    {
        \caption{\textbf{More panoptic segmentation comparison} between \ours with ViT-B backbone and other methods with Swin-B backbone. All backbones are pre-trained on ImageNet-1K with supervised pre-training. \ours still shows competitive results when using only single-scale input.}\label{tab:more_panop}
    }%
\end{table}
  
\boldparagraph{More panoptic segmentation comparison.} Here, we provide more results of \ours with ViT-B backbone and other methods with Swin-B backbone using supervised pre-training on COCO panoptic segmentation in \cref{tab:more_panop}. \ours continues to show strong segmentation performance when using only single-scale input.
